# Supplementary material for: LoD-Loc: Aerial Visual Localization using LoD 3D Map with Neural Wireframe Alignment
Source: arXiv:2410.12269 source file (2024-10-16)
Supplement: Supplementary file 1 [file Additional_Baseline.tex]

% Please add the following required packages to your document preamble:
% \usepackage{multirow}
\begin{table}[h]
\centering
\caption{\textbf{Additional Experiments on Baseline over UAVD4L-LoD dataset.}} %We introduced different baselines, namely eLoFTR, RoMA and Explicit Line Alignment, to demonstrate comparisons with the latest methods. The Explicit Line Alignment method utilizes DeepLSD to extract explicit line segments and construct a distance field, and then refine the final pose based on the distance function. This highlights the necessity of using the feature extractor.}
\label{Tab:AddiBaeline}
\begin{tabularx}{\linewidth}{@{\extracolsep{\fill}}clcccccc}
\toprule
\multicolumn{2}{c}{\multirow{2}{*}{Method}}                 & \multicolumn{3}{c}{\textit{in-Traj.}}                     & \multicolumn{3}{c}{\textit{out-of-Traj.}}                 \\ \cmidrule(r){3-5} \cmidrule(r){6-8} 
\multicolumn{2}{c}{}                                        & 2m-2°           & 3m-3°           & 5m-5°           & 2m-2°           & 3m-3°           & 5m-5°           \\ \midrule
\multirow{2}{*}{\makecell[c]{UAVD4L\\ \textit{Mesh model}} }         & e-LoFTR          & 84.47          & 88.21          & 88.96         & 91.06          & 91.93          & 92.02          \\
                                         & RoMA          & 93.27 & 93.70          &  93.77          & 95.03          & 95.53          & 95.53          \\ \hline
\multirow{2}{*}{ \makecell[c]{CadLoc\\ \textit{LoD model}} } & e-LoFTR          & 0.37              & 0.87              & 1.31              & 0.41              & 0.78              & 1.37              \\
                                         & RoMA          & 2.18              & 2.87              & 3.68              & 6.93              & 8.76              & 10.40               \\ \hline
\multicolumn{2}{c}{\multirow{3}{*}{\makecell[c]{Explicit Line Alignment \\ \textit{LoD model} }}}              & \multirow{3}{*}{10.41}          & \multirow{3}{*}{16.21}          & \multirow{3}{*}{24.19}         & \multirow{3}{*}{6.93}          & \multirow{3}{*}{12.64}          & \multirow{3}{*}{21.62}          \\ \\
\\ \hline
\multirow{2}{*}{\makecell[c]{\textbf{Ours}\\ \textit{LoD model}}}       
                                         & \multirow{2}{*}{Full model}    & \multirow{2}{*}{84.41}          & \multirow{2}{*}{91.77} & \multirow{2}{*}{96.95} & \multirow{2}{*}{95.94} & \multirow{2}{*}{99.00} & \multirow{2}{*}{99.36} \\  \\
\bottomrule
\end{tabularx}
\end{table}
