# Supplementary material for: LoD-Loc: Aerial Visual Localization using LoD 3D Map with Neural Wireframe Alignment
Source: arXiv:2410.12269 source file (2024-10-16)
Supplement: Supplementary file 2 [file Additional_Baseline_epfl.tex]

% Please add the following required packages to your document preamble:
% \usepackage{multirow}
\begin{table}[h]
\centering
\caption{\textbf{Additional Experiments on Baseline over Swiss-EPFL dataset.}} %We introduced different baselines, namely eLoFTR, RoMA and Explicit Line Alignment, to demonstrate comparisons with the latest methods. The Explicit Line Alignment method is the same with Tab~\ref{Tab:AddiBaeline}.}
\label{Tab:AddiBaeline_epfl}
\begin{tabularx}{\linewidth}{@{\extracolsep{\fill}}clcccccc}
\toprule
\multicolumn{2}{c}{\multirow{2}{*}{Method}}                 & \multicolumn{3}{c}{\textit{in-Place.}}                     & \multicolumn{3}{c}{\textit{out-of-Place.}}                 \\ \cmidrule(r){3-5} \cmidrule(r){6-8} 
\multicolumn{2}{c}{}                                        & 2m-2°           & 3m-3°           & 5m-5°           & 2m-2°           & 3m-3°           & 5m-5°           \\ \midrule
\multirow{2}{*}{\makecell[c]{UAVD4L\\ \textit{Mesh model}} }         & e-LoFTR          & 37.64          & 60.96          & 76.40         & 81.53          & 91.03          & 93.93          \\
                                         & RoMA          & 45.98 & 66.77          &  80.73         & 89.18          & 98.68          & 98.94          \\ \hline
\multirow{2}{*}{ \makecell[c]{CadLoc\\ \textit{LoD model}} } & e-LoFTR          & 0              & 0.14              & 0.14              & 0              & 0              & 0.53              \\
                                         & RoMA          & 0.98              & 1.97              & 2.67             & 2.37              & 5.01              & 6.33               \\ \hline
\multicolumn{2}{c}{\multirow{3}{*}{\makecell[c]{Explicit Line Alignment \\ \textit{LoD model} }}}              & \multirow{3}{*}{11.37}          & \multirow{3}{*}{21.35}          & \multirow{3}{*}{33.57}         & \multirow{3}{*}{18.99}          & \multirow{3}{*}{31.39}          & \multirow{3}{*}{45.91}          \\ \\ \\ \hline
\multirow{2}{*}{\makecell[c]{\textbf{Ours}\\ \textit{LoD model}}}       
                                         & \multirow{2}{*}{Full model}    & \multirow{2}{*}{48.60}          & \multirow{2}{*}{65.31} & \multirow{2}{*}{79.78} & \multirow{2}{*}{37.73} & \multirow{2}{*}{57.26} & \multirow{2}{*}{77.57} \\ \\
\bottomrule
\end{tabularx}
\end{table}
