# Supplementary material for: LoD-Loc: Aerial Visual Localization using LoD 3D Map with Neural Wireframe Alignment
Source: arXiv:2410.12269 source file (2024-10-16)
Supplement: Supplementary file 3 [file Additional_explict_align.tex]

% Please add the following required packages to your document preamble:
% \usepackage{multirow}
\begin{table}[htp]
\centering
\caption{\textbf{Additional Experiments on Baseline over UAVD4L-LoD dataset.}}
\label{Tab:AddiBaeline}
\begin{tabularx}{\linewidth}{@{\extracolsep{\fill}}clcccccc}
\toprule
\multicolumn{2}{c}{\multirow{2}{*}{Method}}                 & \multicolumn{3}{c}{\textit{in-Traj.}}                     & \multicolumn{3}{c}{\textit{out-of-Traj.}}                 \\ \cmidrule(r){3-5} \cmidrule(r){6-8} 
\multicolumn{2}{c}{}                                        & 2m-2°           & 3m-3°           & 5m-5°           & 2m-2°           & 3m-3°           & 5m-5°           \\ \midrule
\multirow{2}{*}{\makecell[c]{Explicit\\ \textit{Alignment}} }         & \multirow{2}{*}{Method}          & \multirow{2}{*}{84.47          & \multirow{2}{*}{88.21          & \multirow{2}{*}{88.96         & \multirow{2}{*}{91.06          & \multirow{2}{*}{91.93          & \multirow{2}{*}{92.02          \\
\\
\bottomrule
\end{tabularx}
\end{table}
